# Supplementary material for: Landau-Zener-St\"uckelberg interference in a multimode electromechanical system in the quantum regime
Source: arXiv:1909.07679 ancillary file (2019-09-17)
Supplement: Supplementary file 1 [file HBAR_supplement.pdf]

# Landau-Zener-Stückelberg interference in a multimode electromechanical system in the quantum regime – Supplemental Material

Mikael Kervinen, Alpo Välimaa, and Mika A. Sillanpää*
*Department of Applied Physics, Aalto University, P.O. Box 15100, FI-00076 AALTO, Finland*

Jhon E. Ramírez-Muñoz
*Departamento de Física, Universidad Nacional de Colombia, 111321 Bogotá, Colombia*

## I. TIME-INDEPENDENT EFFECTIVE HAMILTONIAN

Solving the dynamics of the system described by the full Hamiltonian $H(t) = H_{\rm MJC} + H_x(t) + H_z(t)$ is a difficult task because of (i) the multimode nature and (ii) the time dependency. Therefore, it would be much better to derive analytical conditions giving qualitative information of the main features of the system. Particularly, in order to characterize the multiphoton transitions in the driven system, we try to remove the time dependence of the Hamiltonian by performing unitary transformations.

First of all, $H(t)$ is transformed into a rotating frame defined by the excitation frequency, i.e., using $U_1 = \exp\left[i\left(\frac{\sigma_z}{2} + b_i^\dagger b_i\right)\omega_{\rm ext} t\right]$, and considering RWA in the transverse field;

$$H' = \frac{(\omega_0 - \omega_{\rm ext})}{2}\sigma_z + \sum_i (\omega_m^i - \omega_{\rm ext}) b_i^\dagger b_i + \sum_i g_m (b_i\sigma_+ + b_i^\dagger \sigma_-) + \frac{\Omega}{2}\sigma_x + \frac{A}{2}\cos(\omega_{\rm rf} t)\sigma_z. \tag{S1}$$

Subsequently, we apply the unitary transformation $U_2 = \exp\left[i\left(\frac{A}{2\omega_{\rm rf}}\sin(\omega_{\rm rf}t)\sigma_z\right)\right]$, such that the modulation term, $H_z(t)$, is removed from the Hamiltonian: $-i\hbar U_2 \frac{\partial U_2^\dagger}{\partial t} = -H_z(t)$. The Hamiltonian in this non-uniformly rotating frame is:

$$H'' = \frac{(\omega_0 - \omega_{\rm ext})}{2}\sigma_z + \sum_i (\omega_m^i - \omega_{\rm ext}) b_i^\dagger b_i + \sum_i g_m \left(e^{i\frac{A}{\omega_{\rm rf}}\sin(\omega_{\rm rf}t)}\sigma_+ b_i + \text{h.c.}\right) + \frac{\Omega}{2}\left(e^{i\frac{A}{\omega_{\rm rf}}\sin(\omega_{\rm rf}t)}\sigma_+ + \text{h.c.}\right). \tag{S2}$$

After using the Jacobi-Anger expansion, the Hamiltonian yields

$$\begin{aligned} H'' = {} & \frac{(\omega_0 - \omega_{\rm ext})}{2}\sigma_z + \sum_i (\omega_m^i - \omega_{\rm ext}) b_i^\dagger b_i \\ & + \sum_i g_m \sum_{n=-\infty}^{\infty} J_n\left(\frac{A}{\omega_{\rm rf}}\right)\left(\sigma_+ b_i e^{in\omega_{\rm rf}t} + \text{h.c.}\right) \\ & + \frac{\Omega}{2}\sum_{n=-\infty}^{\infty} J_n\left(\frac{A}{\omega_{\rm rf}}\right)\left(\sigma_+ e^{in\omega_{\rm rf}t} + \text{h.c.}\right). \end{aligned} \tag{S3}$$

Now we have time dependency in the qubit-mechanics interaction as well as in the transverse classical field (excitation term). This is removed after moving to the interaction picture with respect to $H_0' = (\omega_0 - \omega_{\rm ext})\sigma_z/2 + \sum_i(\omega_m^i - \omega_{\rm ext}) b_i^\dagger b_i$, and then neglecting all the fast rotating terms, as follows:

$$\begin{aligned} H''_{IP} = {} & \sum_i g_m \sum_{n=-\infty}^{\infty} J_n\left(\frac{A}{\omega_{\rm rf}}\right)\left(\sigma_+ e^{i(\omega_0 - \omega_{\rm ext} + n\omega_{\rm rf})t} b_i e^{-i(\omega_m^i - \omega_{\rm ext})t} + \text{h.c.}\right) \\ & + \frac{\Omega}{2}\sum_{n=-\infty}^{\infty} J_n\left(\frac{A}{\omega_{\rm rf}}\right)\left(\sigma_+ e^{i(\omega_0 - \omega_{\rm ext} + n\omega_{\rm rf})t} + \text{h.c.}\right), \end{aligned} \tag{S4}$$

---

* Mika.Sillanpaa@aalto.fi

which, after make $n \to n-k$ in the first term only, can be rewritten as

$$H''_{IP} = \sum_i g_m \sum_{n=-\infty}^{\infty} J_{n-k}\left(\frac{A}{\omega_{\rm rf}}\right)\left(\sigma_+ e^{i(\omega_0-\omega_{\rm ext}+n\omega_{\rm rf})t} b_i e^{-i(\omega_m^i-\omega_{\rm ext}+k\omega_{\rm rf})t} + \text{h.c.}\right) + \frac{\Omega}{2}\sum_{n=-\infty}^{\infty} J_n\left(\frac{A}{\omega_{\rm rf}}\right)\left(\sigma_+ e^{i(\omega_0-\omega_{\rm ext}+n\omega_{\rm rf})t} + \text{h.c.}\right). \tag{S5}$$

Then we remove the fast oscillating terms by using the transformation

$$V^{(n,k)} = \exp\left[-i\left((\omega_0-\omega_{\rm ext}+n\omega_{\rm rf})\frac{\sigma_z}{2} + \sum_i(\omega_m^i-\omega_{\rm ext}+k\omega_{\rm rf})b_i^\dagger b_i\right)t\right].$$

Finally, the time-independent effective Hamiltonian is a double expansion showing the multiphoton transitions nature for both the qubit and the mechanical modes:

$$H_{\rm eff}^{(n,k)} = \frac{(\omega_0-\omega_{\rm ext}+n\omega_{\rm rf})}{2}\sigma_z + \sum_i(\omega_m^i-\omega_{\rm ext}+k\omega_{\rm rf})b_i^\dagger b_i + \sum_i g_m J_{n-k}\left(\frac{A}{\omega_{\rm rf}}\right)(\sigma_+ b_i + \sigma_- b_i^\dagger) + \frac{\Omega}{2}J_n\left(\frac{A}{\omega_{\rm rf}}\right)\sigma_x. \tag{S6}$$

$H_{\rm eff}^{(n,k)}$ is understood as the interaction between the $n$-order sideband of the qubit and $k$-order sidebands of all the mechanical modes.

## II. NUMERICAL SOLUTION OF THE MASTER EQUATION

If the excitation amplitude to the qubit, $\Omega$, is small in comparison with the decay of the qubit, $\gamma$, the system can be restricted up to the first excitation manifold, and the Hamiltonian for $N$ mechanical modes, becomes:

$$H_{eff}^{(n,k)} = \begin{pmatrix} \bar\omega_m^1 + k\omega_{\rm rf} & & & g_m J_{n-k}(x) & 0 \\ & \bar\omega_m^2 + k\omega_{\rm rf} & & g_m J_{n-k}(x) & 0 \\ & & \ddots & \vdots & \vdots \\ g_m J_{n-k}(x) & g_m J_{n-k}(x) & \cdots & (\bar\omega_0 + n\omega_{\rm rf})/2 & \frac{\Omega}{2}J_n(x) \\ 0 & 0 & \cdots & \frac{\Omega}{2}J_n(x) & -(\bar\omega_0+n\omega_{\rm rf})/2 \end{pmatrix}_{(N+2)\times(N+2)} \tag{S7}$$

with $\bar\omega_m^i = \omega_m^i - \omega_{\rm ext}$, $\bar\omega_0 = \omega_0 - \omega_{\rm ext}$ and $x = A/\omega_{\rm rf}$.

The steady-state population of the qubit can be obtained by solving the master equation including qubit decay:

$$\partial_t\rho = i[\rho, H_{eff}] + \frac{\gamma}{2}\mathcal{L}_{\sigma_-}(\rho) = 0 \tag{S8}$$

with $\mathcal{L}_{\sigma_-}(\rho) = 2\sigma_-\rho\sigma_+ - \{\sigma_+\sigma_-, \rho\}$.

## III. EXPERIMENTAL DATA

In Fig. S1, we focus on the central band of the qubit $n = 0$, where we see diagonal anticrossings. They are separated by the free spectral range $f_{\rm fsr} = 17.4$ MHz. When the modulation frequency is 130-170 MHz we see the interaction of mechanical modes $\omega_m^{(i)}, i = 315 \pm 8, \pm 9, \pm 10$ with the qubit. We also observe in Fig. S1(a) faint lines parallel to the main spectral lines. These are attributed to spurious modes, which are weakly coupled to the qubit at a rate of less than $\frac{1}{10}g_m$. The finding is reproduced in the simulation shown in Fig. S1(b).

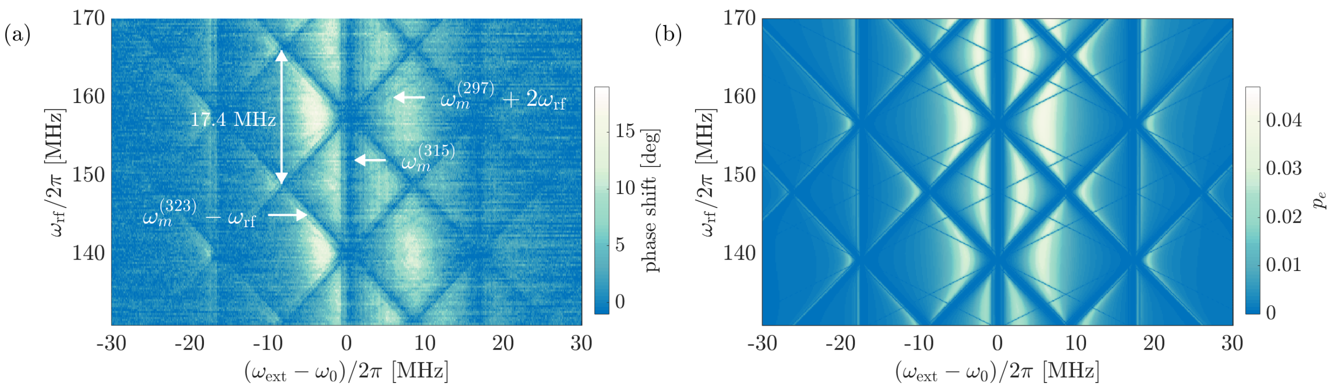


FIG. S1. *Magnification of Figure 5 in the main text.* (a) The measured phase shift, with diagonal lines corresponding to different mechanical modes and their sidebands as labeled. (b) Corresponding numerical simulation of the master equation with $A = 210$ MHz, $\gamma/2\pi = 8$ MHz, $g_m = 5.5$ MHz and $\Omega/2\pi = 3$ MHz.
